# Supplementary material for: Entangling Schr\"odinger's cat states by bridging discrete- and continuous-variable encoding
Source: arXiv:2406.17999 source file (2025-01-21)
Supplement: Supplementary file 1 [file bellCat_supp.pdf]

# Supplementary Information for “Entangling Schrödinger’s cat states by bridging discrete- and continuous-variable encoding”

## 1. DERIVATION OF THE HAMILTONIAN

In this section, we derive the Hamiltonian of two interacting Kerr parametric oscillators (KPOs). The circuit diagram is shown in Supplementary Fig. 1. The Lagrangian of the circuit is given by

$$\mathcal{L} = \mathcal{T} - \mathcal{U},$$

where

$$\begin{aligned} \mathcal{T} &= \left(\frac{\Phi_0}{2\pi}\right)^2 \left[ \frac{C_{s1} + (C_{Ja1} + C_{Jb1})/N_1}{2} \dot{\phi}_1^2 + \frac{C_{s2} + (C_{Ja2} + C_{Jb2})/N_2}{2} \dot{\phi}_2^2 + \frac{C_{\text{int}}}{2} (\dot{\phi}_1 - \dot{\phi}_2)^2 \right] \\ &= \frac{C_{K1}}{2} \dot{\phi}_1^2 + \frac{C_{K2}}{2} \dot{\phi}_2^2 - C_{\text{int}} \dot{\phi}_1 \dot{\phi}_2, \\ \mathcal{U} &= -N_1 E_{Ja1} \cos\left(\frac{\phi_1}{N_1} - r_{a1} \varphi_{\text{ex1}}\right) - N_1 E_{Jb1} \cos\left(\frac{\phi_1}{N_1} + r_{b1} \varphi_{\text{ex1}}\right) \\ &\quad - N_2 E_{Ja2} \cos\left(\frac{\phi_2}{N_2} - r_{a2} \varphi_{\text{ex2}}\right) - N_2 E_{Jb2} \cos\left(\frac{\phi_2}{N_2} + r_{b2} \varphi_{\text{ex2}}\right). \end{aligned}$$

Here,  $\Phi_0$  is the magnetic flux quantum,  $C_{Ki} \equiv (\Phi_0/2\pi)^2 [C_{si} + (C_{Jai} + C_{Jbi})/N_i + C_{\text{int}}]$ ,  $C_{\text{int}} \equiv (\Phi_0/2\pi)^2 C_{\text{int}}$ ,  $\varphi_{\text{ex}i} \equiv 2\pi\Phi_{\text{ex}i}/\Phi_0$ , and  $r_{ai} + r_{bi} = 1$  ( $i = 1, 2$ ), where these scaling parameters are determined by the irrotational constraint [1]. Note that all capacitances are renormalized by a factor of  $(\Phi_0/2\pi)^2$ . Using the formula  $A \cos(x) + B \sin(x) = R \cos(x - \lambda)$ , where  $R = \sqrt{A^2 + B^2}$  and  $\tan(\lambda) = B/A$ , we obtain

$$\mathcal{U} = -N_1 E_{J1} \cos\left(\frac{\phi_1}{N_1} - \lambda_1\right) - N_2 E_{J2} \cos\left(\frac{\phi_2}{N_2} - \lambda_2\right),$$

where

$$\begin{aligned} E_{Ji} &= \sqrt{E_{Jai}^2 + E_{Jbi}^2 + 2E_{Jai}E_{Jbi} \cos(\varphi_{\text{ex}i})}, \\ \lambda_i &= \arctan\left(\frac{E_{Jai} \sin(r_{ai} \varphi_{\text{ex}i}) - E_{Jbi} \sin(r_{bi} \varphi_{\text{ex}i})}{E_{Jai} \cos(r_{ai} \varphi_{\text{ex}i}) + E_{Jbi} \cos(r_{bi} \varphi_{\text{ex}i})}\right). \end{aligned}$$

To account for the flux-bias modulation, we decompose  $\varphi_{\text{ex}i}$  into static and oscillating parts, i.e.,  $\varphi_{\text{dc}i} + \varphi_{\text{ac}i}(t)$ . The oscillating part is the parametric pump given by  $\varphi_{\text{ac}i}(t) = 2\varphi_{\text{ac}i}^{(0)} \cos(\omega_{\text{pi}} t + \theta_{\text{pi}})$ , where  $\omega_{\text{pi}}$  and  $\theta_{\text{pi}}$  are

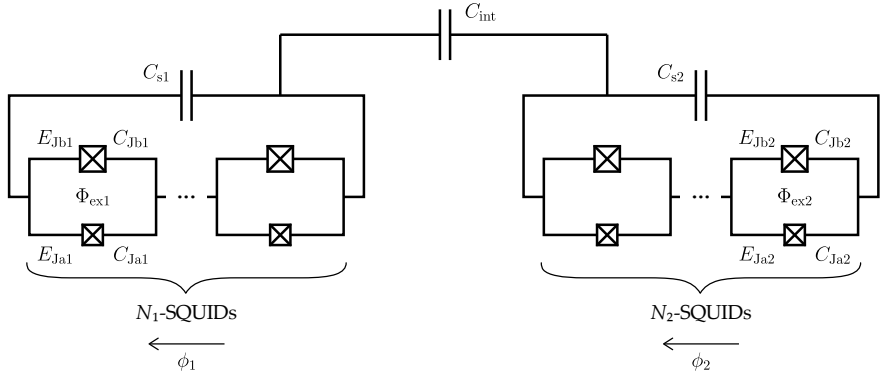

**Supplementary Fig. 1:** Circuit diagram of a superconducting KPO. The KPO consists of  $N_i$  direct-current superconducting quantum interference devices (DC SQUIDS), where  $i = 1, 2$ .  $E_{Jai}$  and  $C_{Jai}$  ( $E_{Jbi}$  and  $C_{Jbi}$ ) represent the Josephson energy and the capacitance of the smaller (larger) junction in each DC SQUID, respectively.  $C_{si}$  denotes the shunting capacitance of the KPO,  $C_{\text{int}}$  is the coupling capacitance between the two KPOs, and  $\Phi_{\text{ex}i}$  is the external magnetic flux threaded through one DC SQUID.

the frequency and phase of the pump applied to KPO<sub>*i*</sub>, respectively. Then, we introduce a variable change,  $\phi_{\text{dci}} \rightarrow \phi_{\text{dci}} + N_i \lambda_i$ . The oscillating part of  $\lambda_i$  is ignored here because the terms associated with it disappear after the rotating-wave approximation [2]. Since  $\varphi_{\text{aci}}^{(0)} \ll 2\pi$ , we take the Taylor expansion at  $\varphi_{\text{exi}} = \varphi_{\text{dci}}$ :

$$\mathcal{U} \approx -N_1 \left( E_{J1}^{(0)} + E_{J1}^{(1)} \varphi_{\text{ac1}} + E_{J1}^{(2)} \varphi_{\text{ac1}}^2 \right) \cos\left(\frac{\phi_1}{N_1}\right) - N_2 \left( E_{J2}^{(0)} + E_{J2}^{(1)} \varphi_{\text{ac2}} + E_{J2}^{(2)} \varphi_{\text{ac2}}^2 \right) \cos\left(\frac{\phi_2}{N_2}\right),$$

where

$$\begin{aligned} E_{Ji}^{(0)} &= \sqrt{E_{Jai}^2 + E_{Jbi}^2 + 2E_{Jai}E_{Jbi}\cos(\varphi_{\text{dci}})}, \\ E_{Ji}^{(1)} &= -\frac{1}{E_{Ji}^{(0)}} E_{Jai}E_{Jbi}\sin(\varphi_{\text{dci}}), \\ E_{Ji}^{(2)} &= -\frac{1}{2(E_{Ji}^{(0)})^3} [E_{Jai}E_{Jbi}(E_{Jai}^2 + E_{Jbi}^2)\cos(\varphi_{\text{dci}}) + (E_{Jai}E_{Jbi})^2\{\cos^2(\varphi_{\text{dci}}) + 1\}]. \end{aligned}$$

Here, the  $\varphi_{\text{aci}}$  terms give the parametric pump, whereas the  $\varphi_{\text{aci}}^2$  terms induce a small frequency shift, which we refer to as an AC Stark-like frequency shift for convenience.

The conjugate number operators are defined by

$$\hbar N_{\phi 1} = \frac{\partial \mathcal{L}}{\partial \dot{\phi}_1} = C_{K1} \dot{\phi}_1 - C_{\text{int}} \dot{\phi}_2, \quad \hbar N_{\phi 2} = \frac{\partial \mathcal{L}}{\partial \dot{\phi}_2} = -C_{\text{int}} \dot{\phi}_1 + C_{K2} \dot{\phi}_2,$$

where the reduced Planck constants are inserted to make  $N_{\phi 1}$  and  $N_{\phi 2}$  dimensionless. In matrix form,

$$\hbar \begin{pmatrix} N_{\phi 1} \\ N_{\phi 2} \end{pmatrix} = \begin{pmatrix} C_{K1} & -C_{\text{int}} \\ -C_{\text{int}} & C_{K2} \end{pmatrix} \begin{pmatrix} \dot{\phi}_1 \\ \dot{\phi}_2 \end{pmatrix}.$$

Using the inverse capacitance matrix, we obtain

$$\begin{pmatrix} \dot{\phi}_1 \\ \dot{\phi}_2 \end{pmatrix} = \frac{\hbar}{C_{K1}C_{K2} - C_{\text{int}}^2} \begin{pmatrix} C_{K2} & C_{\text{int}} \\ C_{\text{int}} & C_{K1} \end{pmatrix} \begin{pmatrix} N_{\phi 1} \\ N_{\phi 2} \end{pmatrix}.$$

The resulting Hamiltonian is (hereafter, we add a hat to an operator for clarity)

$$\begin{aligned} \hat{\mathcal{H}} &= 4E_{C1} \hat{N}_{\phi 1}^2 + 4E_{C2} \hat{N}_{\phi 2}^2 + 8E_{\text{int}} \hat{N}_{\phi 1} \hat{N}_{\phi 2} \\ &\quad - N_1 E_{K1} \cos\left(\frac{\hat{\phi}_1}{N_1}\right) - 2\gamma_1 \cos(\omega_{p1}t + \theta_{p1}) \cos\left(\frac{\hat{\phi}_1}{N_1}\right) - N_2 E_{K2} \cos\left(\frac{\hat{\phi}_2}{N_2}\right) - 2\gamma_2 \cos(\omega_{p2}t + \theta_{p2}) \cos\left(\frac{\hat{\phi}_2}{N_2}\right), \end{aligned}$$

where

$$E_{C1} \equiv \frac{\hbar^2 C_{K2}}{8(C_{K1}C_{K2} - C_{\text{int}}^2)}, \quad E_{C2} \equiv \frac{\hbar^2 C_{K1}}{8(C_{K1}C_{K2} - C_{\text{int}}^2)}, \quad E_{\text{int}} \equiv \frac{\hbar^2 C_{\text{int}}}{8(C_{K1}C_{K2} - C_{\text{int}}^2)}.$$

Here, we define  $E_{Ki} \equiv E_{Ji}^{(0)} + 2E_{Ji}^{(2)}(\varphi_{\text{aci}}^{(0)})^2$  and  $\gamma_i \equiv N_i E_{Ji}^{(1)} \varphi_{\text{aci}}^{(0)}$ . The  $\varphi_{\text{aci}}^2$  term is averaged out by using  $\langle \varphi_{\text{aci}}^2 \rangle = 2(\varphi_{\text{aci}}^{(0)})^2$  and absorbed into  $E_{Ki}$ .

We move to the occupation-number representation by defining

$$\hat{N}_{\phi i} = iN_{\phi i}^{(0)}(\hat{a}_i^\dagger - \hat{a}_i) \quad \text{and} \quad \hat{\phi}_i = \phi_i^{(0)}(\hat{a}_i^\dagger + \hat{a}_i),$$

where  $N_{\phi i}^{(0)} = \sqrt[4]{E_{Ki}/32N_i E_{Ci}}$  and  $\phi_i^{(0)} = \sqrt[4]{2N_i E_{Ci}/E_{Ki}}$  are the zero-point fluctuations. Then we have

$$\begin{aligned} \hat{\mathcal{H}} &= \hbar\omega_{K1}^{(0)} \hat{a}_1^\dagger \hat{a}_1 + \hbar\omega_{K2}^{(0)} \hat{a}_2^\dagger \hat{a}_2 + \hbar g(\hat{a}_1^\dagger \hat{a}_2 + \hat{a}_1 \hat{a}_2^\dagger - \hat{a}_1 \hat{a}_2 - \hat{a}_1^\dagger \hat{a}_2^\dagger) \\ &\quad - N_1 E_{K1} \left[ 1 + \frac{1}{24} \left( \frac{\hat{\phi}_1}{N_1} \right)^4 - \dots \right] - 2\gamma_1 \cos(\omega_{p1}t + \theta_{p1}) \left[ 1 - \frac{1}{2} \left( \frac{\hat{\phi}_1}{N_1} \right)^2 + \frac{1}{24} \left( \frac{\hat{\phi}_1}{N_1} \right)^4 - \dots \right] \\ &\quad - N_2 E_{K2} \left[ 1 + \frac{1}{24} \left( \frac{\hat{\phi}_2}{N_2} \right)^4 - \dots \right] - 2\gamma_2 \cos(\omega_{p2}t + \theta_{p2}) \left[ 1 - \frac{1}{2} \left( \frac{\hat{\phi}_2}{N_2} \right)^2 + \frac{1}{24} \left( \frac{\hat{\phi}_2}{N_2} \right)^4 - \dots \right], \end{aligned}$$

where

$$\hbar\omega_{Ki}^{(0)} \equiv \sqrt{\frac{8E_{Ci}E_{Ki}}{N_i}}, \quad \hbar g \equiv E_{\text{int}} \sqrt{\frac{4E_{K1}E_{K2}}{N_1N_2E_{C1}E_{C2}}} = \frac{1}{2} \frac{E_{\text{int}}}{\sqrt{E_{C1}E_{C2}}} \sqrt{\omega_{K1}^{(0)}\omega_{K2}^{(0)}}. \quad (1)$$

By using the formula (derived on the basis of Ref. [3])

$$(\hat{a}^\dagger \pm \hat{a})^n = \sum_{k=0}^n \sum_{m=0}^{\lfloor \frac{k}{2} \rfloor} \frac{(\pm 1)^{m-k} n!}{(n-k)!(k-2m)!m!2^m} (\hat{a}^\dagger)^{k-2m} \hat{a}^{n-k},$$

we obtain

$$\begin{aligned} -\frac{E_{Ki}}{24N_i^3} \hat{\phi}_i^4 &\Rightarrow -\hbar K_i \hat{a}_i^\dagger \hat{a}_i - \frac{\hbar K_i}{2} \hat{a}_i^\dagger \hat{a}_i^\dagger \hat{a}_i \hat{a}_i \\ &\quad - \frac{\hbar K_i}{12} \left( 6\hat{a}_i^\dagger \hat{a}_i^\dagger + 6\hat{a}_i \hat{a}_i + 4\hat{a}_i^\dagger \hat{a}_i \hat{a}_i \hat{a}_i + 4\hat{a}_i^\dagger \hat{a}_i^\dagger \hat{a}_i \hat{a}_i + \hat{a}_i \hat{a}_i \hat{a}_i \hat{a}_i + \hat{a}_i^\dagger \hat{a}_i^\dagger \hat{a}_i^\dagger \hat{a}_i \right), \\ \frac{\gamma_i}{N_i^2} \cos(\omega_{pi}t + \theta_{pi}) \hat{\phi}_i^2 &\Rightarrow \hbar P_i \cos(\omega_{pi}t + \theta_{pi}) \left( 2\hat{a}_i^\dagger \hat{a}_i + \hat{a}_i^\dagger \hat{a}_i^\dagger + \hat{a}_i \hat{a}_i \right), \end{aligned} \quad (2)$$

where  $\hbar K_i \equiv E_{Ci}/N_i^2$  and  $\hbar P_i \equiv \varphi_{aci}^{(0)} E_{ji}^{(1)} \sqrt{2E_{Ci}/N_i E_{Ki}}$ .

Now we move to the rotating frame whose Hamiltonian is defined by

$$\hat{\mathcal{H}}_0/\hbar = \frac{\omega_{p1}}{2} \hat{a}_1^\dagger \hat{a}_1 + \frac{\omega_{p2}}{2} \hat{a}_2^\dagger \hat{a}_2$$

and make the rotating-wave approximation. Then, the surviving terms are

$$\begin{aligned} \hat{\mathcal{H}}_{\text{rot}}/\hbar &= e^{i\hat{\mathcal{H}}_0 t/\hbar} (\hat{\mathcal{H}} - \hat{\mathcal{H}}_0) e^{-i\hat{\mathcal{H}}_0 t/\hbar} \times (1/\hbar) \\ &\approx \Delta_1 \hat{a}_1^\dagger \hat{a}_1 - \frac{K_1}{2} \hat{a}_1^\dagger \hat{a}_1^\dagger \hat{a}_1 \hat{a}_1 + \frac{P_1}{2} \left( \hat{a}_1^\dagger \hat{a}_1^\dagger + \hat{a}_1 \hat{a}_1 \right) + \Delta_2 \hat{a}_2^\dagger \hat{a}_2 - \frac{K_2}{2} \hat{a}_2^\dagger \hat{a}_2^\dagger \hat{a}_2 \hat{a}_2 + \frac{P_2}{2} \left( \hat{a}_2^\dagger \hat{a}_2^\dagger + \hat{a}_2 \hat{a}_2 \right) \\ &\quad + g \left[ \hat{a}_1^\dagger \hat{a}_2 e^{+i(\Delta_p t + \theta_p)} + \hat{a}_1 \hat{a}_2^\dagger e^{-i(\Delta_p t + \theta_p)} \right]. \end{aligned} \quad (3)$$

Here,  $\Delta_i (\equiv \omega_{Ki} - \omega_{pi}/2)$  is the KPO-pump frequency detuning, where  $\omega_{Ki} (\equiv \omega_{Ki}^{(0)} - K_i)$  is the transition frequency between the  $|0_F\rangle$  and  $|1_F\rangle$  states;  $\Delta_p \equiv (\omega_{p1} - \omega_{p2})/2$  and  $\theta_p \equiv (\theta_{p1} - \theta_{p2})/2$ . Note that the unitary transformation  $\hat{a}_i \rightarrow \hat{a}_i e^{-i\theta_{pi}/2}$  was performed. Setting  $\theta_p = 0$  gives Eq. (1) in the main text.

## 2. SYSTEM PARAMETERS

The measured system parameters are presented in Supplementary Table 1. The Hamiltonian was characterized by analysing Rabi oscillations in the  $|0_F\rangle$  state population, following the methodology outlined in Ref. [6], except for the coupling constant  $g$ . The value of  $g$  was determined by tuning the global flux bias to the point where the transition frequency of both KPOs becomes equal and then observing the anti-crossing in the KPO signal. At this flux bias, where  $\omega_{K1}/2\pi = \omega_{K2}/2\pi = 2.237$  GHz,  $g/2\pi$  was found to be 7.2 MHz. Consequently, the coupling constant at our working flux bias, where  $\omega_{K1}/2\pi = 2.564$  GHz and  $\omega_{K2}/2\pi = 2.420$  GHz, would be 8.0 MHz, according to Supplementary Eq. (1).

The calibration between the AWG setting value and the displacement in phase space was achieved by fitting the parity measurement of the vacuum state with the following Hamiltonian [5, 6]:

$$\begin{aligned} \hat{\mathcal{H}}_{\text{fit}}/\hbar &= \Delta_{Ki} \hat{a}_i^\dagger \hat{a}_i - \frac{K_i}{2} \hat{a}_i^\dagger \hat{a}_i^\dagger \hat{a}_i \hat{a}_i + \beta_i \left( \hat{a}_i^\dagger e^{-i\Delta_{\text{dT}i} t} + \hat{a}_i e^{+i\Delta_{\text{dT}i} t} \right) \\ &\quad + \hbar \Delta_{Ti} \hat{b}_i^\dagger \hat{b}_i - \frac{K_{Ti}}{2} \hat{b}_i^\dagger \hat{b}_i^\dagger \hat{b}_i \hat{b}_i + \beta_{Ti} (\hat{b}_i^\dagger + \hat{b}_i) + \chi_{KTi} \hat{a}_i^\dagger \hat{a}_i \hat{b}_i^\dagger \hat{b}_i + \chi_{KKTi} \hat{a}_i^\dagger \hat{a}_i (\hat{a}_i^\dagger \hat{a}_i - 1) \hat{b}_i^\dagger \hat{b}_i. \end{aligned} \quad (4)$$

Here,  $\Delta_{Ki} \equiv \omega_{Ki} - \omega_{\text{Tdi}}$ , where  $\omega_{\text{Tdi}}$  is the frequency of the drive for transmon  $i$  ( $i = 1, 2$ );  $\Delta_{\text{dT}i} \equiv \omega_{di} - \omega_{\text{Tdi}}$ ; and  $\Delta_{Ti} \equiv \omega_{Ti} - \omega_{\text{Tdi}}$ . For more details, see Ref. [6].

**Supplementary Table 1:** Measured system parameters.  $\Phi_0$  is the magnetic flux quantum. “RR” stands for readout resonator. For the self-Kerr coefficient of the KPOs, the value in parentheses is the coefficient when the pump is on. For more rigorous definitions, see Supplementary Eqs. (3) and (4).

| Physical quantity                                                           | Symbol                    | System 1                  | System 2                  |
|-----------------------------------------------------------------------------|---------------------------|---------------------------|---------------------------|
| Number of DC SQUIDs in KPO                                                  | $N_i$                     | 10                        | 10                        |
| External magnetic flux threaded through one DC SQUID                        | $\Phi_{\text{ex}i}$       | $0.229\Phi_0$             | $0.191\Phi_0$             |
| Transition frequency between the $ 0\rangle$ and $ 1\rangle$ states of KPO  | $\omega_{\text{Ki}}/2\pi$ | 2.5635 GHz                | 2.4199 GHz                |
| Self-Kerr coefficient of KPO                                                | $K_i/2\pi$                | 2.86 (2.05) MHz           | 2.91 (1.90) MHz           |
| Longitudinal relaxation time of KPO                                         | $T_1^{\text{Ki}}$         | $13 \pm 3 \mu\text{s}$    | $20 \pm 6 \mu\text{s}$    |
| Transverse relaxation time of KPO                                           | $T_2^{\text{Ki}}$         | $4.8 \pm 0.4 \mu\text{s}$ | $4.3 \pm 0.8 \mu\text{s}$ |
| Coupling constant between two KPOs                                          | $g/2\pi$                  | 8.0 MHz                   |                           |
| Transition frequency between $ g\rangle$ and $ e\rangle$ states of transmon | $\omega_{\text{Ti}}/2\pi$ | 3.8076 GHz                | 3.6216 GHz                |
| Anharmonicity of transmon                                                   | $K_{\text{Ti}}/2\pi$      | 221.3 MHz                 | 225.9 MHz                 |
| Longitudinal relaxation time of transmon                                    | $T_1^{\text{Ti}}$         | $49 \pm 7 \mu\text{s}$    | $37 \pm 4 \mu\text{s}$    |
| Transverse relaxation time of transmon                                      | $T_2^{\text{Ti}}$         | $25 \pm 2 \mu\text{s}$    | $13 \pm 1 \mu\text{s}$    |
| Cross-Kerr coefficient between KPO and transmon                             | $\chi_{\text{KT}i}/2\pi$  | 1.69 MHz                  | 1.72 MHz                  |
| Higher-order cross-Kerr coefficient                                         | $\chi_{\text{KKT}i}/2\pi$ | −7 kHz                    | −7 kHz                    |
| Number of thermally excited photons in KPO                                  | $n_{\text{th}i}$          | 0.09                      | 0.08                      |
| Resonance frequency of RR                                                   | $\omega_{\text{R}i}/2\pi$ | 7.6079 GHz                | 7.4641 GHz                |
| Cross-Kerr coefficient between transmon and RR                              | $\chi_{\text{TR}i}/2\pi$  | 0.37 MHz                  | 0.39 MHz                  |

### 3. FULL PULSE SEQUENCE

The full pulse sequence, including that for Wigner-function measurement via the Lutterbach–Davidovich method [7–9], is depicted in Supplementary Fig. 2. Specific details regarding pulse shapes are outlined in Supplementary Table 2. Notably, a 340 ns delay is introduced between the displacement pulse for KPO1 and the first  $\pi/2$  pulse for transmon1 to prevent the unintended excitation of transmon1 triggered by the  $\pi/2$  pulses for transmon2. This precaution is necessary owing to the small frequency difference (only 35 MHz) between the  $|e\rangle$ – $|f\rangle$  transition of transmon1 and the  $|g\rangle$ – $|e\rangle$  transition of transmon2, falling within the bandwidth of the  $\pi/2$  pulses for Wigner function measurement. By comparing two one-mode Wigner function measurements of KPO1—one obtained from the simultaneous measurement of both transmons with the delay, and the other from the transmon1 measurement only without the delay—we found that this delay does not severely degrade the quality of the Wigner function measurement, as the Kerr evolution preserves the number parity.

### 4. SIMULATION OF BELL–CAT STATE GENERATION

#### A. Conversion from Fock to cat

We simulate our Bell–Cat generation scheme via conversion from Fock states to cat states by solving the following Lindblad master equation with QuTiP [10, 11]:

$$\frac{\partial \rho(t)}{\partial t} = -\frac{i}{\hbar}[\hat{\mathcal{H}}(t), \rho(t)] + \{\gamma_{\text{K}1}\mathcal{D}[\hat{a}_1] + \gamma_{\text{K}2}\mathcal{D}[\hat{a}_2] + \gamma_{\phi 1}\mathcal{D}[\hat{a}_1^\dagger \hat{a}_1] + \gamma_{\phi 2}\mathcal{D}[\hat{a}_2^\dagger \hat{a}_2]\}\rho(t), \quad (5)$$

where  $\rho$  is the density matrix of the two-KPO system,  $\mathcal{D}[\hat{O}]\rho = \hat{O}\rho\hat{O}^\dagger - \frac{1}{2}\hat{O}^\dagger\hat{O}\rho - \frac{1}{2}\rho\hat{O}^\dagger\hat{O}$ ,  $\gamma_{\text{K}i}$  is the single-photon loss rate of KPO $i$ , and  $\gamma_{\phi i}$  is the dephasing rate of KPO $i$  ( $i = 1, 2$ ).

We first simulate the Bell–Fock state preparation. In a frame rotating with the frequency  $\omega_{\text{K}1}$ , the Hamiltonian describing the Bell-preparation pulse for the  $|0_{\text{F}}1_{\text{F}}\rangle \pm |1_{\text{F}}0_{\text{F}}\rangle$  state is given by

$$\begin{aligned} \hat{\mathcal{H}}_{\text{BFd}}/\hbar = & -\frac{K_1}{2}\hat{a}_1^\dagger\hat{a}_1^\dagger\hat{a}_1\hat{a}_1 + (\omega_{\text{K}2} - \omega_{\text{K}1})\hat{a}_2^\dagger\hat{a}_2 - \frac{K_2}{2}\hat{a}_2^\dagger\hat{a}_2^\dagger\hat{a}_2\hat{a}_2 \\ & + g(\hat{a}_1^\dagger\hat{a}_2 + \hat{a}_1\hat{a}_2^\dagger) + 2P_g \cos[(\omega_{\text{K}1} - \omega_{\text{K}2} + \delta_g)t + \theta_g] \hat{a}_1^\dagger\hat{a}_1. \end{aligned} \quad (6)$$

Here,  $P_g$  and  $\theta_g$  represent the amplitude and phase of the pulse, respectively. The factor of 2 preceding  $P_g$  originates from Supplementary Eq. (2). A small detuning,  $\delta_g/2\pi = 0.88$  MHz, was used in the simulation to align the pulse frequency with the centre frequency of the Rabi pattern.

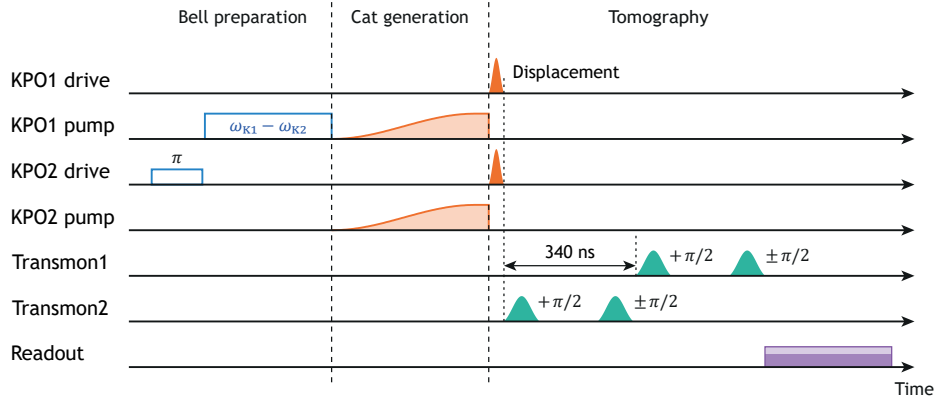

**Supplementary Fig. 2:** Full pulse sequence of Fig. 2c. In the “tomography” part, the displacement pulses applied to both KPOs implement the displacement operators described in Eqs. (2) and (3) in the main text. The subsequent  $\pi/2$  pulses applied to the transmons map the number parity of the KPOs to the transmon states. Then, the states of the two transmons are measured simultaneously. For this measurement, two microwave pulses with the frequencies of the readout resonators are combined and applied to the chip. Regarding the 340 ns delay in the transmon1 pulse sequence, see the supplementary text.

**Supplementary Table 2:** Parameters for the pulse shape. “ $\sigma$ ” represents the standard deviation of Gaussian pulses. For flap-top Gaussian pulses,  $\sigma$  indicates the standard deviation of the pulse edges. The time intervals between two  $\pi/2$  transmon pulses for the parity measurement are 278 ns for KPO1 and 280 ns for KPO2.

| Operation                                  | Data                                             | Element           | Pulse shape                         | Pulse length (ns) | $\sigma$ (ns) |
|--------------------------------------------|--------------------------------------------------|-------------------|-------------------------------------|-------------------|---------------|
| Cat generation                             | Figs. 1–3                                        | KPO               | $\sin^2(\pi t/2\tau_{\text{ramp}})$ | 1000              |               |
| Bell preparation                           | Fig. 2 ( $ 0_F 1_F\rangle$ )                     | KPO2              | Flat-top Gaussian                   | 955               | 1             |
|                                            | Fig. 2 ( $ 0_F 1_F\rangle \pm  1_F 0_F\rangle$ ) | KPO1              | Flat-top Gaussian                   | 730               | 1             |
|                                            | Fig. 2 ( $ 0_F 0_F\rangle \pm  1_F 1_F\rangle$ ) | KPO1              | Flat-top Gaussian                   | 852               | 1             |
| Two-cat Rabi<br>$\sqrt{\text{iSWAP}}$ gate | Fig. 3                                           | KPO1              | Flat-top Gaussian                   | Variable          | 1             |
|                                            |                                                  |                   |                                     | 275               | 1             |
| Parity measurement                         | All Wigner functions                             | KPO               | Gaussian                            | 10                | 2.5           |
|                                            |                                                  | Transmon          | Gaussian ( $\pi/2$ )                | 25                | 6.25          |
| Rabi                                       | Fig. 4                                           | KPO               | Flat-top Gaussian                   | Variable          | 1             |
|                                            |                                                  | Transmon          | Gaussian ( $\pi$ )                  | 2000              | 500           |
| Transmon readout                           | All data                                         | Readout resonator | Flat-top Gaussian                   | 2500              | 4             |

The  $|0_F 0_F\rangle \pm |1_F 1_F\rangle$  state preparation can also be simulated similarly by using the following Hamiltonian in a frame rotating with the frequency  $(\omega_{K1} + \omega_{K2})/2$ :

$$\begin{aligned}
 \hat{\mathcal{H}}_{\text{BFs}}/\hbar = & \left( \frac{\omega_{K1} - \omega_{K2}}{2} + \delta_g \right) \hat{a}_1^\dagger \hat{a}_1 - \frac{K_1}{2} \hat{a}_1^\dagger \hat{a}_1^\dagger \hat{a}_1 \hat{a}_1 + \left( \frac{\omega_{K2} - \omega_{K1}}{2} + \delta_g \right) \hat{a}_2^\dagger \hat{a}_2 - \frac{K_2}{2} \hat{a}_2^\dagger \hat{a}_2^\dagger \hat{a}_2 \hat{a}_2 \\
 & + g \left( \hat{a}_1^\dagger \hat{a}_2 + \hat{a}_1 \hat{a}_2^\dagger \right) + \frac{P_g}{2} \left( \hat{a}_1^\dagger \hat{a}_1^\dagger e^{-i\theta_g} + \hat{a}_1 \hat{a}_1 e^{i\theta_g} \right),
 \end{aligned} \tag{7}$$

where  $\delta_g/2\pi = -30$  kHz in our simulation.

Next, we simulate the cat generation process by solving Supplementary Eq. (5) with Supplementary Eq. (3), using the result of the Bell–Fock preparation simulation with Eq. (6) or (7) as the initial state. The coupling term in Supplementary Eq. (3) was omitted at this step because, without a Bell-preparation or gate pulse, its contribution would be averaged out.

Supplementary Table 3 summarises the infidelity between the measured and target states due to thermal excitation, single-photon loss, and dephasing estimated through these simulations. Two-mode Wigner functions for the target states and selected simulated states are presented in Supplementary Figs. 3 and 4, respectively.

**Supplementary Table 3:** Impact of error sources on the fidelity between the measured and target states. The values represent infidelities estimated through simulations that selectively included or excluded the Lindblad operators in Eq. (5). The column labelled “Thermal excitation” indicates the infidelity between the vacuum state and the tensor-product thermal states of both KPOs, while “Imperfect operation” reflects infidelity due to imperfect control arising from the small Kerr coefficient. For cat generation process, dephasing is not considered because low-frequency noise does not affect the fidelity as pointed out in the main text. Values from Supplementary Tables 1 and 2 were used for the simulation. In our simulations, these infidelities were found to be additive. Consequently, the resulting fidelity of the simulated Bell–Cat states ranges from 0.66 to 0.70, depending on the presence of the  $\pi$ -pulse. Em dashes denote “not applicable.”

| Step                     | Thermal excitation | Single-photon loss | Dephasing | Imperfect operation |
|--------------------------|--------------------|--------------------|-----------|---------------------|
| Vacuum state preparation | 0.14               | —                  | —         | —                   |
| $\pi$ -pulse on KPO2     | —                  | 0.01               | 0.02      | 0.01                |
| Bell preparation         | —                  | 0.01               | 0.02      | 0.01                |
| Cat generation           | —                  | 0.08               | —         | 0.03                |

### B. Two-cat gate operation

To simulate two-cat Rabi oscillations, it is convenient to express the Hamiltonian for our two-cat gate operation in the following form [4]:

$$\hat{\mathcal{H}}_g/\hbar = 2P_g \cos(\omega_g t + \theta_g) \hat{a}_1^\dagger \hat{a}_1 = 2P_g \cos[(\Delta_p + \Delta_g)t + \theta_g] \hat{a}_1^\dagger \hat{a}_1, \quad (8)$$

where  $\Delta_g \equiv \omega_g - \Delta_p$ . The results in Fig. 5a were obtained using Supplementary Eqs. (3), (8), and (5).

## 5. TWO-CAT RABI OSCILLATIONS IN INTERACTING TWO-LEVEL SYSTEM QUBITS

As mentioned in the main text, the two-cat Rabi oscillations can be reproduced in interacting two-level qubits, whose resonance frequencies are  $\omega_{q1}$  and  $\omega_{q2}$ . We first consider  $|0_F 1_F\rangle \leftrightarrow |1_F 0_F\rangle$  transitions induced by the parametric modulation of the coupling constant with the frequency  $\omega_g$ . The Hamiltonian describing this process is given by [12]

$$\hat{\mathcal{H}}_{Rs}/\hbar = J_g \cos[(\Delta_q + \Delta_g)t] (\hat{\sigma}_+^{(1)} \hat{\sigma}_-^{(2)} e^{+i\Delta_q t} + \hat{\sigma}_-^{(1)} \hat{\sigma}_+^{(2)} e^{-i\Delta_q t}), \quad (9)$$

where  $J_g$  is the modulation amplitude of the coupling constant,  $\Delta_q \equiv \omega_{q1} - \omega_{q2}$ ,  $\Delta_g \equiv \omega_g - \Delta_q$ , and  $\hat{\sigma}_\pm^{(k)} \equiv (\hat{\sigma}_x^{(k)} \pm i\hat{\sigma}_y^{(k)})/2$ , where  $\hat{\sigma}_x^{(k)}$  and  $\hat{\sigma}_y^{(k)}$  are the Pauli operators of qubit  $k$  ( $k = 1, 2$ ). To reproduce our data for  $|0_C 1_C\rangle \leftrightarrow |1_C 0_C\rangle$  transitions, we need two modulation tones with opposite detuning:

$$\hat{\mathcal{H}}_{Rd}/\hbar = \frac{J_g}{2} [\cos\{(\Delta_q + \Delta_g)t\} + \cos\{(\Delta_q - \Delta_g)t\}] (\hat{\sigma}_+^{(1)} \hat{\sigma}_-^{(2)} e^{+i\Delta_q t} + \hat{\sigma}_-^{(1)} \hat{\sigma}_+^{(2)} e^{-i\Delta_q t}). \quad (10)$$

Here, the frequency  $\Delta_q + \Delta_g$  corresponds to  $\omega_g$  and the frequency  $\Delta_q - \Delta_g$  corresponds to  $2(\omega_{q1} - \omega_{q2}) - \omega_g$ . The simulations using Supplementary Eqs. (9) and (10) are shown in Supplementary Fig. 5b.

## 6. TWO-CAT GATE OPERATION IN MATRIX FORM

Here, we present the mathematical form of our two-cat gate operation. The gate, originally proposed in Ref. [4], corresponds to an  $\hat{R}_{ZZ}(2\Theta)$  operation in the coherent-state basis  $|\pm\alpha\rangle$ , which we denote as  $|0_\alpha\rangle$  and  $|1_\alpha\rangle$ , respectively:

$$\hat{R}_{ZZ}(2\Theta) = \begin{matrix} |0_\alpha 0_\alpha\rangle \\ |0_\alpha 1_\alpha\rangle \\ |1_\alpha 0_\alpha\rangle \\ |1_\alpha 1_\alpha\rangle \end{matrix} \begin{pmatrix} \langle 0_\alpha 0_\alpha | & \langle 0_\alpha 1_\alpha | & \langle 1_\alpha 0_\alpha | & \langle 1_\alpha 1_\alpha | \\ e^{-i\Theta} & & & \\ & e^{i\Theta} & & \\ & & e^{i\Theta} & \\ & & & e^{-i\Theta} \end{pmatrix}.$$

In the coherent state basis, the cat-state basis is expressed as follows:

$$\begin{aligned} |0_C 0_C\rangle &= \frac{1}{2}(|0_\alpha 0_\alpha\rangle + |0_\alpha 1_\alpha\rangle + |1_\alpha 0_\alpha\rangle + |1_\alpha 1_\alpha\rangle) \\ |0_C 1_C\rangle &= \frac{1}{2}(|0_\alpha 0_\alpha\rangle - |0_\alpha 1_\alpha\rangle + |1_\alpha 0_\alpha\rangle - |1_\alpha 1_\alpha\rangle) \\ |1_C 0_C\rangle &= \frac{1}{2}(|0_\alpha 0_\alpha\rangle + |0_\alpha 1_\alpha\rangle - |1_\alpha 0_\alpha\rangle - |1_\alpha 1_\alpha\rangle) \\ |1_C 1_C\rangle &= \frac{1}{2}(|0_\alpha 0_\alpha\rangle - |0_\alpha 1_\alpha\rangle - |1_\alpha 0_\alpha\rangle + |1_\alpha 1_\alpha\rangle) \end{aligned}$$

Thus, the transformation between the coherent- and cat-state basis for an arbitrary wavefunction  $|\psi\rangle$  is given by

$$\begin{pmatrix} \langle 0_C 0_C | \psi \rangle \\ \langle 0_C 1_C | \psi \rangle \\ \langle 1_C 0_C | \psi \rangle \\ \langle 1_C 1_C | \psi \rangle \end{pmatrix} = \underbrace{\frac{1}{2} \begin{pmatrix} 1 & 1 & 1 & 1 \\ 1 & -1 & 1 & -1 \\ 1 & 1 & -1 & -1 \\ 1 & -1 & -1 & 1 \end{pmatrix}}_{\hat{U}_T} \begin{pmatrix} \langle 0_\alpha 0_\alpha | \psi \rangle \\ \langle 0_\alpha 1_\alpha | \psi \rangle \\ \langle 1_\alpha 0_\alpha | \psi \rangle \\ \langle 1_\alpha 1_\alpha | \psi \rangle \end{pmatrix},$$

where  $\hat{U}_T$  is the transformation matrix.

The  $\hat{R}_{ZZ}$  gate in the cat-state basis is expressed as

$$\hat{U}_G = \hat{U}_T^\dagger \hat{R}_{ZZ}(2\Theta) \hat{U}_T = \begin{pmatrix} \langle 0_C 0_C | & \langle 0_C 1_C | & \langle 1_C 0_C | & \langle 1_C 1_C | \\ |0_C 0_C\rangle & |0_C 1_C\rangle & |1_C 0_C\rangle & |1_C 1_C\rangle \end{pmatrix} \begin{pmatrix} \cos(\Theta) & & & -i \sin(\Theta) \\ & \cos(\Theta) & -i \sin(\Theta) & \\ & -i \sin(\Theta) & \cos(\Theta) & \\ -i \sin(\Theta) & & & \cos(\Theta) \end{pmatrix}.$$

Equation (2) in the main text is obtained by setting  $\Theta = -\pi/4$ .

## 7. ELECTRONICS AND CABLING

The pulses for the transmon and the readout resonator were generated by arbitrary waveform generators (AWGs), local oscillators, and IQ mixers. For the KPO, pulses were generated using Keysight M8195A (labelled “Fast AWG” in Supplementary Fig. 6a). This instrument has four channels, with each channel having two outputs, such as Ch. 1 and Ch.  $\bar{1}$  (see the leftmost part of Supplementary Fig. 6a). The pulse shapes from these two outputs are identical, with only a  $180^\circ$  phase difference. In Ch. 1 (and Ch.  $\bar{1}$ ), both the KPO1 drive and low-frequency pulses near the frequency  $(\omega_{K1} - \omega_{K2})/2\pi = 144$  MHz are generated. The pulses from Ch. 1 pass through a bandpass filter to suppress the low-frequency component, while the pulses from Ch.  $\bar{1}$  pass through multiple low-pass filters to cut out the gigahertz components. The KPO1 pump and the low-frequency pulses are combined in the mixing chamber and inserted into the KPO1 pump port of the chip (Fig. 1c).

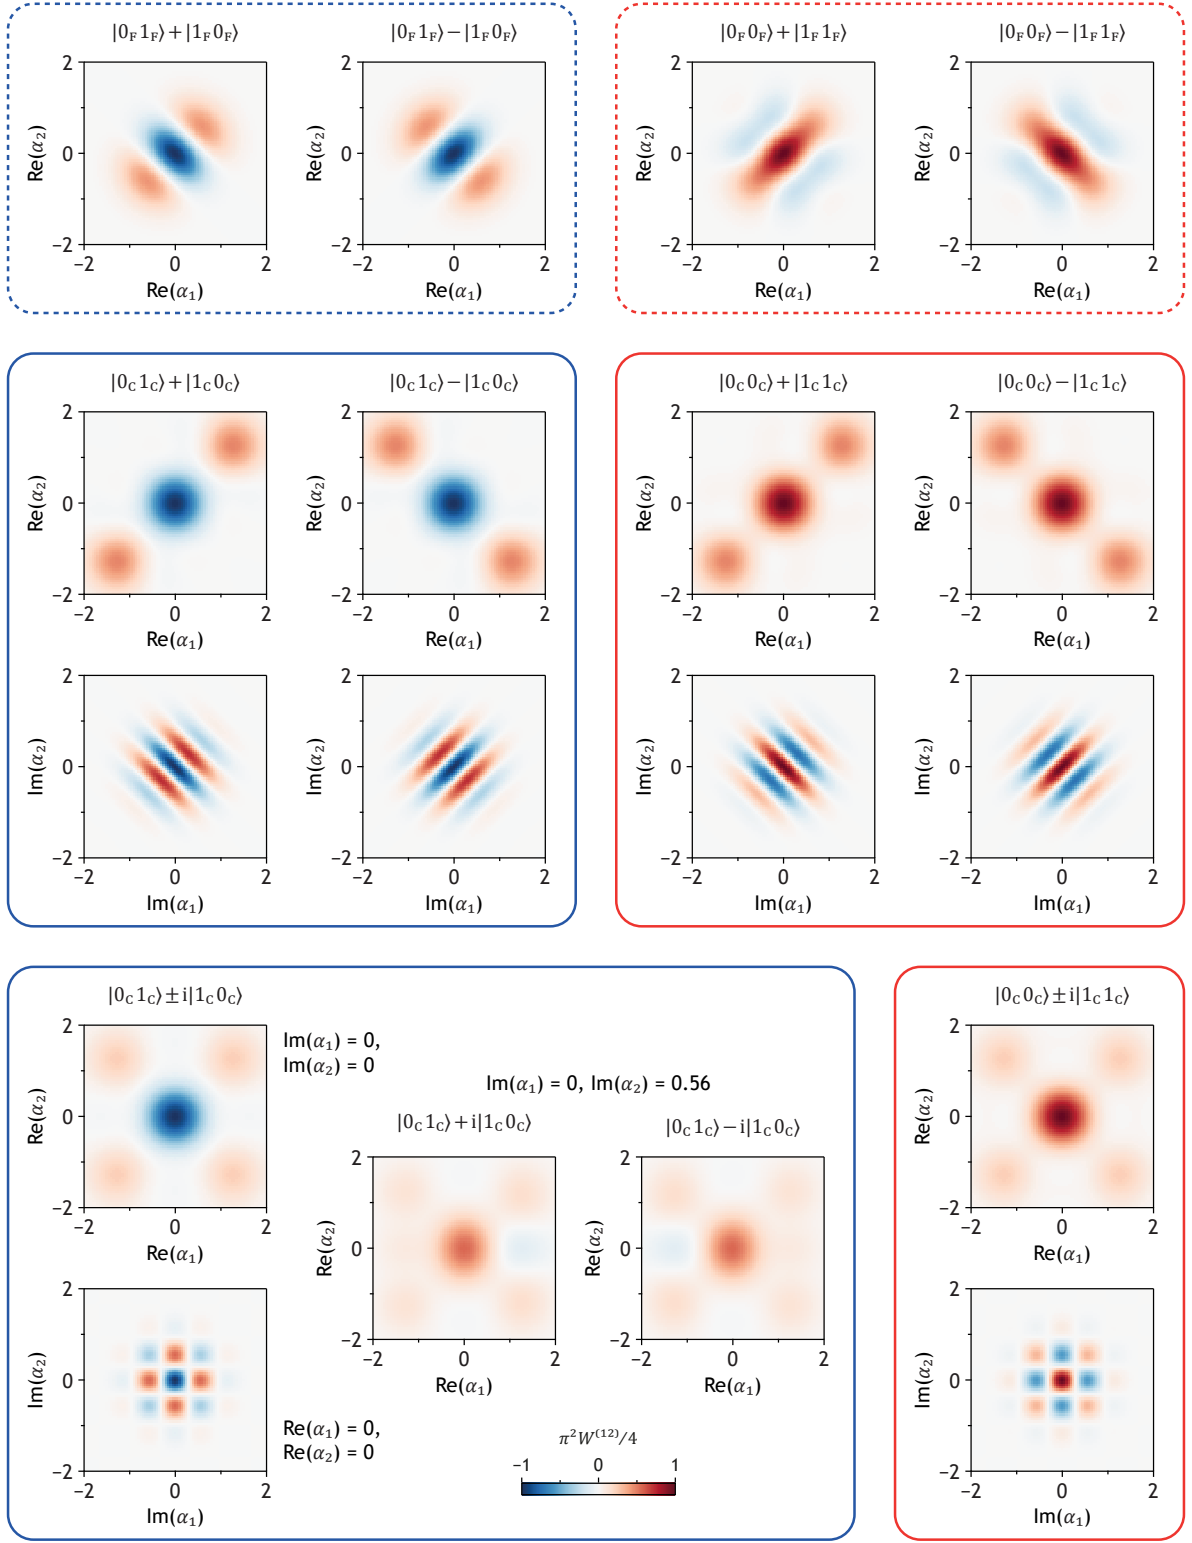

**Supplementary Fig. 3:** Two-mode Wigner functions of our target states. The cat states are eigenstates with the conditions  $P_i = K_i$  and  $\Delta_i = 0.5K_i$  ( $i = 1, 2$ ). For Re-Re plots,  $\text{Im}(\alpha_1) = \text{Im}(\alpha_2) = 0$ , unless otherwise specified; for Im-Im plots,  $\text{Re}(\alpha_1) = \text{Re}(\alpha_2) = 0$ .

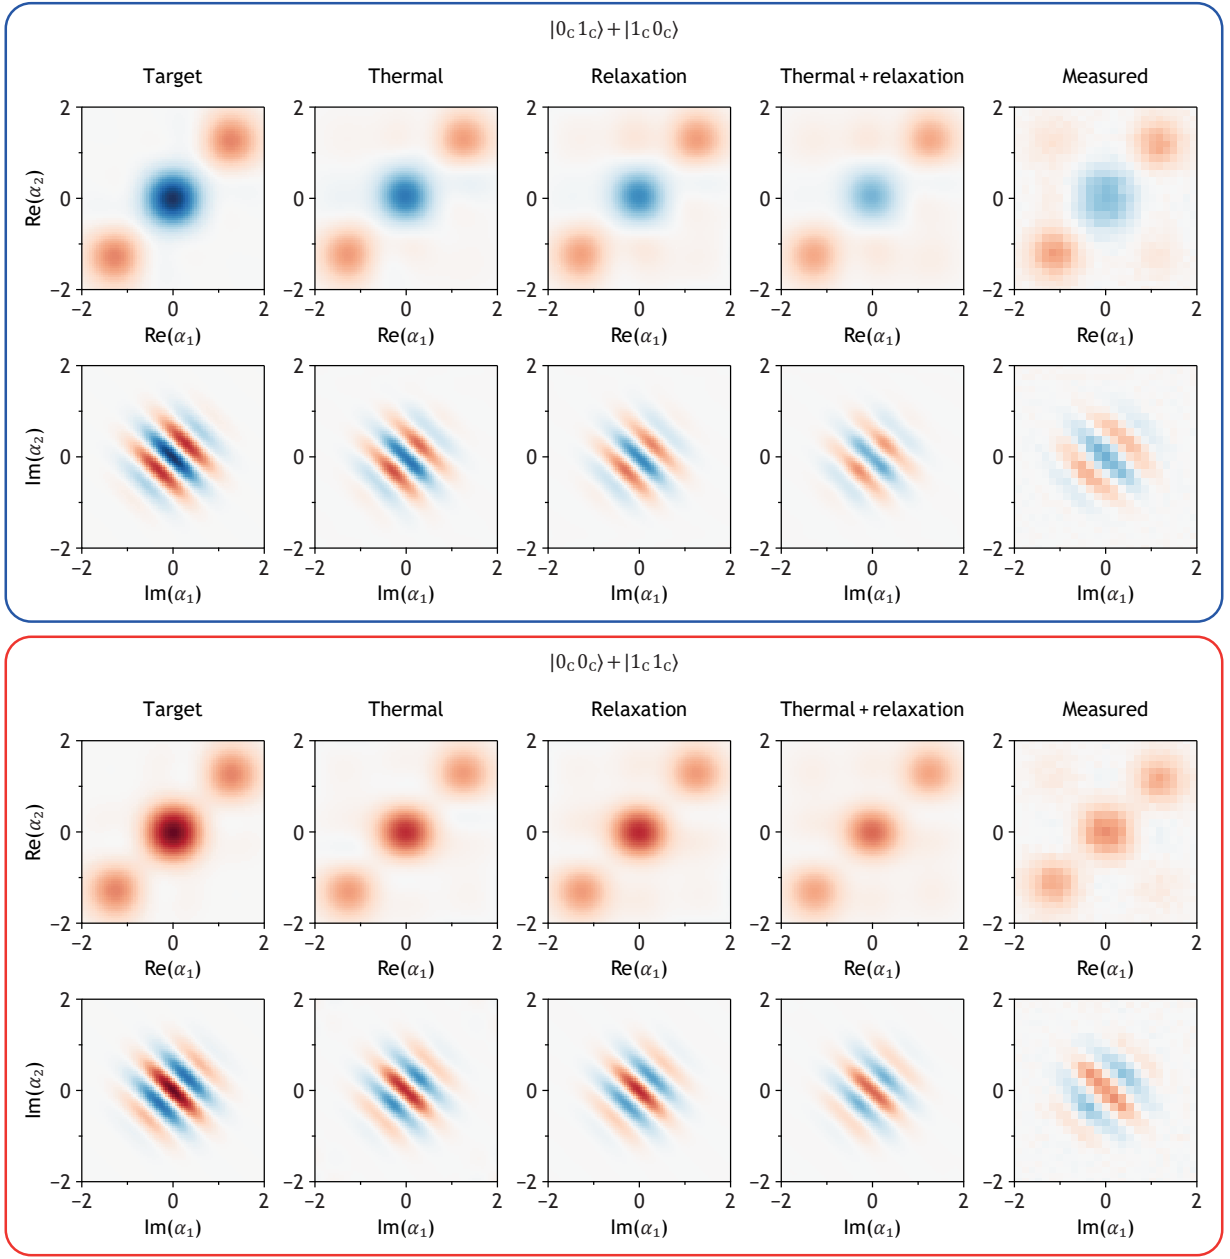

**Supplementary Fig. 4:** Two-mode Wigner functions for the target state (“Target”); simulated states with thermal states as initial states (“Thermal”), relaxation effects such as single-photon loss and dephasing (“Relaxation”), or both (“Thermal + relaxation”); and our measured results (“Measured”).

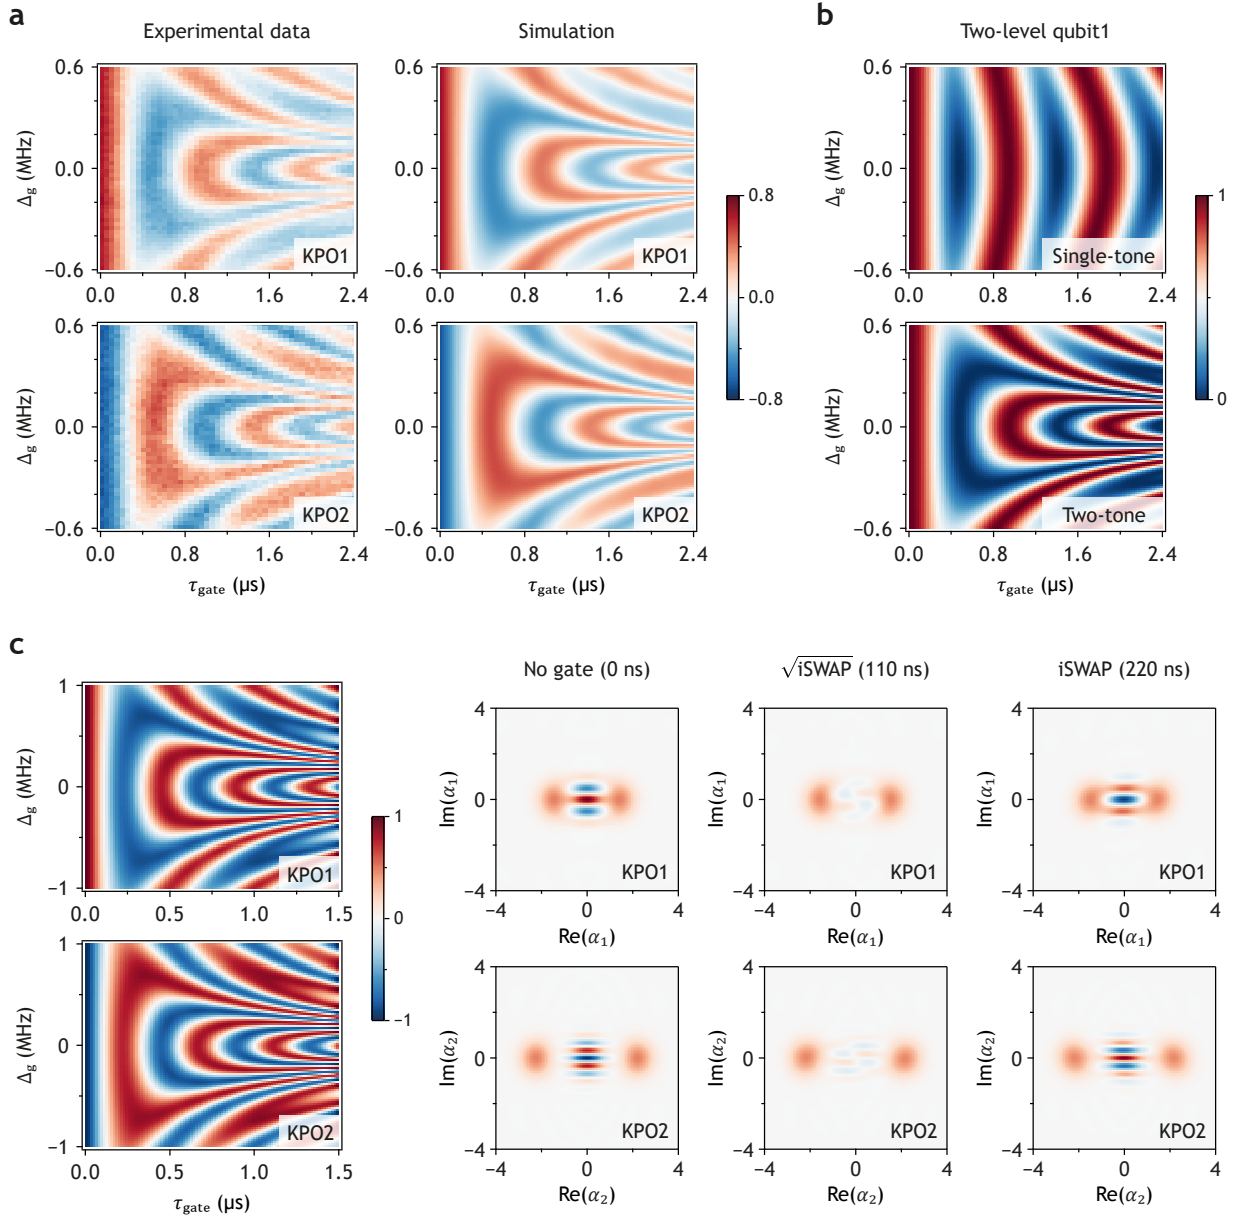

**Supplementary Fig. 5:** **a** Two-cat Rabi oscillations. The colours represent the number parity of each KPO. The gate amplitude from the fitting with the simulation is 2.96 MHz. In the simulation, both  $T_1^{K1}$  and  $T_1^{K2}$  were assumed 10  $\mu\text{s}$ ; dephasing was not considered. For more details, see Sec. 4B. **b** Simulation of Rabi oscillations in two interacting two-level qubits. The colours represent the population of the  $|0\rangle$  state of qubit1. For this simulation, Supplementary Eqs. (9) (single tone) and (10) (two tones) with  $J_m/2\pi = 1.06$  MHz were used. **c** Two-cat Rabi oscillations between two KPOs with different mean photon numbers. The mean photon number of KPO1 is 2.1, whereas that of KPO2 is 5.1. For the simulation, Supplementary Eqs. (3), (8), and (5) were used with the following conditions: The Kerr coefficient for both KPOs is 2 MHz; the pump amplitude and detuning for KPO1 are 3 MHz and 1 MHz, respectively; for KPO2, 8 MHz and 2 MHz, respectively. Relaxations are not considered in (b) and (c).



# SUPPLEMENTARY REFERENCES

- [1] X. You, J. A. Sauls, and J. Koch, *Circuit quantization in the presence of time-dependent external flux*, Phys. Rev. B **99**, 174512 (2019).
- [2] C. W. S. Chang, C. Sabín, P. Forn-Díaz, F. Quijandría, A. M. Vadiraj, I. Nsanzineza, G. Johansson, and C. M. Wilson, *Observation of Three-Photon Spontaneous Parametric Down-Conversion in a Superconducting Parametric Cavity*, Phys. Rev. X **10**, 011011 (2020).
- [3] W. Wyss, *Two Non-Commutative Binomial Theorems*, Preprint at <https://doi.org/10.48550/arXiv.1707.03861> (2017).
- [4] H. Chono, T. Kanao, and H. Goto, *Two-qubit gate using conditional driving for highly detuned Kerr nonlinear parametric oscillators*, Phys. Rev. Research **4**, 043054 (2022).
- [5] A. Essig, Q. Ficheux, T. Peronnin, N. Cottet, R. Lescanne, A. Sarlette, P. Rouchon, Z. Leghtas, and B. Huard, *Multiplexed Photon Number Measurement*, Phys. Rev. X **11**, 031045 (2021).
- [6] D. Iyama, T. Kamiya, S. Fujii, H. Mukai, Y. Zhou, T. Nagase, A. Tomonaga, R. Wang, J.-J. Xue, S. Watabe, S. Kwon, and J.-S. Tsai, *Observation and manipulation of quantum interference in a superconducting Kerr parametric oscillator*, Nat. Commun. **15**, 86 (2024).
- [7] L. G. Lutterbach and L. Davidovich, *Method for Direct Measurement of the Wigner Function in Cavity QED and Ion Traps*, Phys. Rev. Lett. **78**, 2547 (1997).
- [8] S. Haroche and J.-M. Raimond, *Exploring the Quantum: Atoms, Cavities, and Photons* (Oxford University Press, 2006).
- [9] B. Vlastakis, G. Kirchmair, Z. Leghtas, S. E. Nigg, L. Frunzio, S. M. Girvin, M. Mirrahimi, M. H. Devoret, and R. J. Schoelkopf, *Deterministically Encoding Quantum Information Using 100-Photon Schrödinger Cat States*, Science **342**, 607–610 (2013).
- [10] J. R. Johansson, P. D. Nation, and F. Nori, *QuTiP: An open-source Python framework for the dynamics of open quantum systems*, Comp. Phys. Comm. **183**, 1760–1772 (2012).
- [11] J. R. Johansson, P. D. Nation, and F. Nori, *QuTiP 2: A Python framework for the dynamics of open quantum systems*, Comp. Phys. Comm. **184**, 1234–1240 (2013).
- [12] S. Kwon, A. Tomonaga, G. L. Bhai, S. J. Devitt, and J.-S. Tsai, *Gate-based superconducting quantum computing*, J. Appl. Phys. **129**, 041102 (2021).
